# Supplementary material for: Nuclear-electronic orbital second-order coupled cluster for excited states
Source: arXiv:2509.17977 source file (2025-09-22)
Supplement: Supplementary file 1 [file CC2_SuppMat.pdf]

# Supplementary Material

## Nuclear–electronic orbital second-order coupled cluster for excited states

Jonathan H. Fetherolf<sup>†</sup>, Fabijan Pavošević<sup>‡</sup> and Sharon Hammes-Schiffer<sup>\*,†</sup>

<sup>†</sup>*Department of Chemistry, Princeton University, Princeton, NJ 08544, United States*

<sup>‡</sup>*Algorithmiq Ltd., FI-00160 Helsinki, Finland*

E-mail: shs566@princeton.edu

### Contents

|                                                                          |    |
|--------------------------------------------------------------------------|----|
| S1 NEO-CC2 excited-state Jacobian equations                              | S2 |
| S2 Protonic excitations with alternative electron-proton scaling factors | S5 |
| S3 HCN with different conventional basis sets                            | S6 |
| References                                                               | S7 |

## S1 NEO-CC2 excited-state Jacobian equations

Excited states of the NEO-CC2 Hamiltonian are obtained within coupled cluster response theory via diagonalization of the Jacobian matrix

$$\begin{aligned} \mathbf{A}_{\mu_i \nu_j} &= \frac{\partial \Omega_{\mu_i}}{\partial a_{\nu_j}} = \begin{pmatrix} \mathbf{A}_{\mu_1 \nu_1} & \mathbf{A}_{\mu_1 \nu_2} \\ \mathbf{A}_{\mu_2 \nu_1} & \mathbf{A}_{\mu_2 \nu_2} \end{pmatrix} \\ &= \begin{pmatrix} \langle 0_e 0_p | a_{\mu_1} ([\bar{H} + [\bar{H}, \hat{T}_2]), a_{\nu_1}] | 0_e 0_p \rangle & \langle 0_e 0_p | a_{\mu_1} [\bar{H}, a_{\nu_2}] | 0_e 0_p \rangle \\ \langle 0_e 0_p | a_{\mu_2} [\bar{H}, a_{\nu_1}] | 0_e 0_p \rangle & \langle 0_e 0_p | a_{\mu_2} [\hat{F}, a_{\nu_2}] | 0_e 0_p \rangle \end{pmatrix} \end{aligned} \quad (\text{S1})$$

composed of the singles-singles, singles-doubles, doubles-singles and doubles-doubles blocks. These blocks can be written in terms of electronic molecular orbitals denoted by indices  $i, j, k, l$  for occupied and  $a, b, c, d$  for unoccupied, and protonic molecular orbitals denoted by indices  $I, J, K, L$  for occupied and  $A, B, C, D$  for unoccupied. The singles-singles, singles-doubles, doubles-singles and doubles-doubles blocks, respectively, are

$$\mathbf{A}_{\mu_1 \nu_1} = \begin{pmatrix} \mathbf{A}_{ia, kc} & \mathbf{A}_{ia, KC} \\ \mathbf{A}_{ia, KC} & \mathbf{A}_{IA, KC} \end{pmatrix}, \quad (\text{S2a})$$

$$\mathbf{A}_{\mu_1 \nu_2} = \begin{pmatrix} \mathbf{A}_{ia, kcld} & \mathbf{A}_{ia, kcKC} \\ \mathbf{A}_{IA, kcld} & \mathbf{A}_{IA, kcKC} \end{pmatrix}, \quad (\text{S2b})$$

$$\mathbf{A}_{\mu_2 \nu_1} = \begin{pmatrix} \mathbf{A}_{iajb, kc} & \mathbf{A}_{iajb, KC} \\ \mathbf{A}_{iaIA, kc} & \mathbf{A}_{iaIA, KC} \end{pmatrix}, \quad (\text{S2c})$$

$$\mathbf{A}_{\mu_2 \nu_2} = \begin{pmatrix} \mathbf{A}_{iajb, kcld} & \mathbf{A}_{iajb, kcKC} \\ \mathbf{A}_{iaIA, kcld} & \mathbf{A}_{iaIA, kcKC} \end{pmatrix}. \quad (\text{S2d})$$

The programmable equations for these matrix elements are given below for spin free (spatial) orbitals in the restricted electronic case.

$$\begin{aligned}
A_{ia,kc} = & \delta_k^i F_a^c - \delta_a^c F_k^i - g_{ak}^{ci} + 2g_{ak}^{ic} - \delta_k^i F_{i1}^c t_a^{i1} + 2\delta_k^i t_{a1}^{i1} g_{ai1}^{ca1} - \delta_k^i t_{a1}^{i1} g_{ai1}^{a1c} \\
& - \delta_k^i t_{A1}^{I1} g_{aI1}^{cA1} - 2\delta_k^i t_{aa1}^{i1i2} g_{i1i2}^{ca1} + \delta_k^i t_{aa1}^{i1i2} g_{i1i2}^{a1c} + \delta_k^i t_{aA1}^{i1I1} g_{i1I1}^{cA1} - 2\delta_k^i t_a^{i1} t_{a1}^{i2} g_{i1i2}^{ca1} \\
& + \delta_k^i t_a^{i1} t_{a1}^{i2} g_{i1i2}^{a1c} + \delta_k^i t_a^{i1} t_{A1}^{I1} g_{i1I1}^{cA1} - \delta_a^c F_k^{a1} t_{a1}^i - 2\delta_a^c t_{a1}^{i1} g_{ki1}^{ia1} + \delta_a^c t_{a1}^{i1} g_{ki1}^{a1i} \\
& + \delta_a^c t_{A1}^{I1} g_{kI1}^{iA1} + \delta_a^c t_{a1A1}^{I1} g_{kI1}^{a1A1} - 2\delta_a^c t_{a1a2}^{ii1} g_{ki1}^{a1a2} + \delta_a^c t_{a1a2}^{i1i} g_{ki1}^{a1a2} - 2\delta_a^c t_{a1}^{i1} t_{a2}^{i1} g_{ki1}^{a1a2} \\
& + \delta_a^c t_{a1}^{i1} t_{a2}^{i1} g_{ki1}^{a2a1} + \delta_a^c t_{a1}^{i1} t_{A1}^{I1} g_{kI1}^{a1A1} - 2t_a^{i1} g_{ki1}^{ci} + t_a^{i1} g_{ki1}^{ic} - t_{a1}^i g_{ak}^{ca1} + 2t_{a1}^i g_{ak}^{a1c} \\
& + 4t_{aa1}^{ii1} g_{ki1}^{ca1} - 2t_{aa1}^{i1i} g_{ki1}^{ca1} - 2t_{aa1}^{ii1} g_{ki1}^{a1c} + t_{aa1}^{i1i} g_{ki1}^{a1c} - 2t_{aA1}^{I1} g_{kI1}^{cA1} - 2t_a^{i1} t_{a1}^i g_{ki1}^{ca1} \\
& + t_a^{i1} t_{a1}^i g_{ki1}^{a1c}
\end{aligned} \tag{S3}$$

$$\begin{aligned}
A_{IA,KC} = & \delta_K^I F_A^C - \delta_A^C F_K^I - \delta_K^I F_{I1}^C t_A^{I1} - \delta_A^C F_K^{A1} t_{A1}^I + 2\delta_A^C t_{a1}^{i1} g_{i1K}^{a1I} - 2\delta_K^I t_{a1}^{i1} g_{i1A}^{a1C} \\
& + 2\delta_A^C t_{a1A1}^{i1I} g_{i1K}^{a1A1} + 2\delta_K^I t_{a1A1}^{i1I1} g_{i1I1}^{a1C} - 2t_{a1}^{i1} g_{i1K}^{a1C} + 2\delta_K^I t_{a1A}^{i1I1} g_{i1I1}^{a1C} \\
& + 2\delta_K^I t_{a1}^{i1} t_A^{I1} g_{i1I1}^{a1C} + 2\delta_K^I t_{a1}^{i1} t_{A1}^I g_{i1K}^{a1A1}
\end{aligned} \tag{S4}$$

$$A_{ia,KC} = -g_{aK}^{iC} + t_a^{i1} g_{i1K}^{iC} - t_{a1}^i g_{aK}^{a1C} - 2t_{aa1}^{ii1} g_{i1K}^{a1C} + t_{aa1}^{i1i} g_{i1K}^{a1C} + t_{a1}^i t_a^{i1} g_{i1K}^{a1C} \tag{S5}$$

$$A_{IA,kc} = -g_{kA}^{cI} - t_{A1}^I g_{kA}^{cA1} + t_A^{I1} g_{kI1}^{cI} - t_{a1A}^{i1I} g_{ki1}^{a1c} + 2t_{a1A}^{i1I} g_{ki1}^{ca1} + t_{A1}^I t_A^{I1} g_{kI1}^{cA1} \tag{S6}$$

$$\begin{aligned}
A_{iajb,kc} = & \delta_k^i g_{ab}^{cj} + \delta_k^j g_{ab}^{ic} - \delta_b^c g_{ak}^{ij} - \delta_a^c g_{bk}^{ji} + \delta_k^i t_{a1}^j g_{ab}^{ca1} - \delta_k^i t_b^{i1} g_{ai1}^{cj} - \delta_k^i t_a^{i1} g_{bi1}^{jc} \\
& - \delta_k^i t_b^{i1} t_{a1}^j g_{ai1}^{ca1} - \delta_k^i t_a^{i1} t_{a1}^j g_{bi1}^{a1c} + \delta_k^i t_a^{i1} t_b^{i2} g_{i1i2}^{cj} + \delta_k^i t_a^{i1} t_b^{i2} t_{a1}^j g_{i1i2}^{ca1} \\
& + \delta_k^j t_{a1}^i g_{ab}^{a1c} - \delta_k^j t_b^{i1} g_{ai1}^{ic} - \delta_k^j t_a^{i1} g_{bi1}^{ci} - \delta_k^j t_b^{i1} t_{a1}^i g_{ai1}^{a1c} - \delta_k^j t_a^{i1} t_{a1}^i g_{bi1}^{ca1} \\
& + \delta_k^j t_a^{i1} t_b^{i2} g_{i1i2}^{ic} + \delta_k^j t_a^{i1} t_b^{i2} t_{a1}^i g_{i1i2}^{a1c} - \delta_b^c t_{a1}^j g_{ak}^{ia1} - \delta_b^c t_{a1}^j g_{ak}^{a1j} + \delta_b^c t_a^{i1} g_{ki1}^{ji} \\
& - \delta_b^c t_a^{i1} t_{a1}^j g_{ak}^{a1a2} + \delta_b^c t_a^{i1} t_{a1}^j g_{ki1}^{ja1} + \delta_b^c t_a^{i1} t_{a1}^j g_{ki1}^{a1i} + \delta_b^c t_a^{i1} t_{a1}^j t_{a2}^j g_{ki1}^{a2a1} \\
& - \delta_a^c t_{a1}^i g_{bk}^{ja1} - \delta_a^c t_{a1}^j g_{bk}^{a1i} + \delta_a^c t_b^{i1} g_{ki1}^{ij} - \delta_a^c t_r^{i1} t_{a2}^j g_{bk}^{a2a1} + \delta_a^c t_b^{i1} t_{a1}^j g_{ki1}^{ia1} \\
& + \delta_a^c t_b^{i1} t_{a1}^j g_{ki1}^{a1j} + \delta_a^c t_b^{i1} t_{a1}^j t_{a2}^j g_{ki1}^{a1a2}
\end{aligned} \tag{S7}$$

$$\begin{aligned}
A_{ia,kcld} = & \delta_a^d \delta_l^i F_k^c - \frac{1}{2} \delta_a^c \delta_l^i F_k^d - \frac{1}{2} \delta_a^d \delta_k^i F_l^c + \delta_a^c \delta_k^i F_l^d - \frac{1}{2} \delta_l^i g_{ak}^{cd} + \delta_l^i g_{ak}^{dc} + \delta_k^i g_{al}^{cd} \\
& - \frac{1}{2} \delta_k^i g_{al}^{dc} - \delta_a^d g_{kl}^{ci} + \frac{1}{2} \delta_a^c g_{kl}^{di} + \frac{1}{2} \delta_a^d g_{kl}^{ic} - \delta_a^c g_{kl}^{id} - \delta_a^d t_{a1}^i g_{kl}^{ca1} + \frac{1}{2} \delta_a^d t_{a1}^i g_{kl}^{a1c} \\
& - \delta_a^c t_{a1}^i g_{kl}^{a1d} + \frac{1}{2} \delta_a^c t_{a1}^i g_{kl}^{da1} - \delta_l^i t_a^{i1} g_{ki1}^{cd} + \frac{1}{2} \delta_l^i t_a^{i1} g_{ki1}^{dc} + 2 \delta_l^i \delta_a^d t_{a1}^{i1} g_{ki1}^{ca1} \\
& - \delta_l^i \delta_a^d t_{a1}^{i1} g_{ki1}^{a1c} - \delta_l^i \delta_a^d t_{A1}^{I1} g_{kI1}^{cA1} - \delta_l^i \delta_a^c t_{a1}^{i1} g_{ki1}^{da1} - \frac{1}{2} \delta_l^i \delta_a^c t_{a1}^{i1} g_{ki1}^{a1d} + \frac{1}{2} \delta_l^i \delta_a^c t_{A1}^{I1} g_{kI1}^{dA1} \\
& - \delta_k^i t_a^{i1} g_{li1}^{dc} + \frac{1}{2} \delta_k^i t_a^{i1} g_{li1}^{cd} - \delta_k^i \delta_a^d t_{a1}^{i1} g_{li1}^{ca1} + \frac{1}{2} \delta_k^i \delta_a^d t_{a1}^{i1} g_{li1}^{a1c} + \frac{1}{2} \delta_k^i \delta_a^d t_{A1}^{I1} g_{lI1}^{cA1} \\
& - \delta_k^i \delta_a^c t_{a1}^{i1} g_{li1}^{a1d} + 2 \delta_k^i \delta_a^c t_{a1}^{i1} g_{li1}^{da1} - \delta_k^i \delta_a^c t_{A1}^{I1} g_{lI1}^{dA1}
\end{aligned} \tag{S8}$$

$$A_{ia,kcKC} = \delta_a^c \delta_k^i F_K^C + \delta_a^c g_{kK}^{iC} - \delta_k^i g_{aK}^{cC} + \delta_k^i t_a^{i1} g_{i1K}^{cC} - 2 \delta_a^c \delta_k^i t_{a1}^{i1} g_{i1K}^{a1C} + \delta_a^c t_{a1}^i g_{kK}^{a1C} \tag{S9}$$

$$\begin{aligned}
A_{IA,kcKC} = & 2 \delta_A^C \delta_K^I F_k^c + 2 \delta_A^C g_{kK}^{cI} - 2 \delta_K^I g_{kA}^{cC} + 4 \delta_A^C \delta_K^I t_{a1}^{i1} g_{ki1}^{ca1} - 2 \delta_A^C \delta_K^I t_{a1}^{i1} g_{ki1}^{a1c} \\
& - 2 \delta_A^C \delta_K^I t_{A1}^{I1} g_{kI1}^{cA1} + 2 \delta_K^I t_A^{I1} g_{kI1}^{cC} + 2 \delta_A^C t_{A1}^I g_{kK}^{cA1}
\end{aligned} \tag{S10}$$

$$\begin{aligned}
A_{iaIA,kc} = & \delta_a^c g_{kA}^{iI} - \delta_k^i g_{aA}^{cI} + \delta_a^c t_{a1}^i g_{kA}^{a1I} - \delta_a^c t_{A1}^I g_{kA}^{iA1} - \delta_k^i t_{A1}^I g_{aA}^{cA1} - \delta_a^c t_A^{I1} g_{kI1}^{iI} \\
& + \delta_k^i t_A^{I1} g_{aI1}^{cI} + \delta_k^i t_a^{i1} g_{i1A}^{cI} + \delta_a^c t_{a1}^i t_{A1}^I g_{kA}^{a1A1} + \delta_k^i t_a^{i1} t_{A1}^I g_{i1A}^{cA1} - \delta_a^c t_{a1}^i t_A^{I1} g_{kI1}^{a1I} \\
& - \delta_a^c t_{A1}^I t_A^{I1} g_{kI1}^{iA1} + \delta_k^i t_a^{i1} t_A^{I1} g_{i1I1}^{cI} - \delta_k^i t_{A1}^I t_A^{I1} g_{aI1}^{cA1} - \delta_a^c t_{a1}^i t_{A1}^I t_A^{I1} g_{kI1}^{a1A1} \\
& - \delta_k^i t_a^{i1} t_{A1}^I t_A^{I1} g_{i1I1}^{cA1}
\end{aligned} \tag{S11}$$

$$\begin{aligned}
A_{iaIA,KC} = & \delta_A^C g_{aK}^{iI} - \delta_K^I g_{aA}^{iC} - \delta_K^I t_{a1}^i g_{aA}^{a1C} + \delta_A^C t_{a1}^i g_{aK}^{a1I} + \delta_A^C t_{A1}^I g_{aK}^{iA1} - \delta_A^C t_a^{i1} g_{i1K}^{iI} \\
& + \delta_K^I t_A^{I1} g_{aI1}^{iC} + \delta_K^I t_a^{i1} g_{i1A}^{iC} + \delta_A^C t_{a1}^i t_{A1}^I g_{aK}^{a1A1} + \delta_K^I t_{a1}^i t_A^{I1} g_{aI1}^{a1C} - \delta_A^C t_{a1}^i t_a^{i1} g_{i1K}^{a1I} \\
& + \delta_K^I t_{a1}^i t_a^{i1} g_{i1A}^{a1C} - \delta_A^C t_a^{i1} t_{A1}^I g_{i1K}^{iA1} - \delta_K^I t_a^{i1} t_A^{I1} g_{i1I1}^{iC} - \delta_A^C t_a^{i1} t_{A1}^I t_A^{I1} g_{i1K}^{a1A1} \\
& - \delta_K^I t_{a1}^i t_a^{i1} t_A^{I1} g_{i1I1}^{a1C}
\end{aligned} \tag{S12}$$

$$A_{iajb,KC} = A_{IA,kcld} = A_{iaIA,kcld} = A_{iajb,kcKC} = 0 \tag{S13}$$

$$A_{iajb,kcld} = \delta_k^i \delta_a^c \delta_l^j \delta_b^d (F_a^c + F_b^d - F_k^i - F_l^j) \tag{S14}$$

$$A_{iaIA,kcKC} = \delta_k^i \delta_a^c \delta_K^I \delta_A^C (F_a^c + F_A^C - F_k^i - F_K^I) \tag{S15}$$

## S2 Protonic excitations with alternative electron-proton scaling factors

Table S1, Table S2, and Fig. S1 are identical to Table III, Table IV, and Fig. 1 from the main text, but with NEO-SOS'-CC2 electron-proton scaling factors  $c_{\text{ep}}^{\text{gs}} = 1.0$  and  $c_{\text{ep}}^{\text{ex}} = 8.0$ .

Table S1: Energies of lowest-lying excited states for  $\text{HeHHe}^+$ . The states are labeled according to quanta in the protonic vibrational modes  $(\nu_1, \nu_2, \nu_3)$ , where  $\nu_1$  and  $\nu_2$  are degenerate bending modes and  $\nu_3$  is the stretching mode. The NEO-SOS'-CC2 results are given with scaling factors  $c_{\text{ep}}^{\text{gs}} = 1.0$  and  $c_{\text{ep}}^{\text{ex}} = 8.0$ . All energies are given in  $\text{cm}^{-1}$ .

| Method                                      | (1,0,0)/(0,1,0) | (2,0,0)/(0,2,0) | (1,1,0) | (0,0,1) |
|---------------------------------------------|-----------------|-----------------|---------|---------|
| FGH Reference <sup>a</sup>                  | 772             | 1584            | 1619    | 1818    |
| NEO-MR-SDT <sub>een</sub> CI <sup>a,b</sup> | 723             | 1654            | 1784    | 2371    |
| NEO-TDDFT <sup>c</sup>                      | 611             | 5366            | 5490    | 2211    |
| NEO-CC2 <sup>b</sup>                        | 1030            | 2407            | 2442    | 2388    |
| NEO-SOS'-CC2 <sup>b</sup>                   | 778             | 2383            | 2106    | 2098    |

<sup>a</sup> Obtained from Ref. 1.

<sup>b</sup> Computed with aug-cc-pVTZ/0.4404-def2-QZVP\*/8s8p8d8f8g basis set.

<sup>c</sup> Computed with aug-cc-pVTZ/cc-pV6Z/8s8p8d8f8g basis set.

Table S2: First four protonic excited states of HCN. The NEO-SOS'-CC2 results are given with scaling factors  $c_{\text{ep}}^{\text{gs}} = 1.0$  and  $c_{\text{ep}}^{\text{ex}} = 8.0$ . All values are given in  $\text{cm}^{-1}$ .

| Method                                      | (1,0,0)/(0,1,0) | (1,1,0) | (2,0,0)/(0,2,0) | (0,0,1) |
|---------------------------------------------|-----------------|---------|-----------------|---------|
| FGH Reference <sup>a</sup>                  | 634             | 1261    | 1277            | 3173    |
| NEO-MR-SDT <sub>een</sub> CI <sup>b,c</sup> | 678             | —       | —               | 2968    |
| NEO-TDDFT <sup>d</sup>                      | 681             | 5801    | 7262            | 3118    |
| NEO-CC2 <sup>c</sup>                        | 1223            | 2970    | 3038            | 3121    |
| NEO-SOS'-CC2 <sup>c</sup>                   | 851             | 2818    | 2938            | 2886    |

<sup>a</sup> Obtained from Ref. 2.

<sup>b</sup> Obtained from Ref. 1.

<sup>c</sup> Computed using cc-pVTZ/0.1393-def2-QZVP\*/8s8p8d8f basis.

<sup>d</sup> Computed using cc-pVTZ/cc-pV6Z/8s8p8d8f basis.

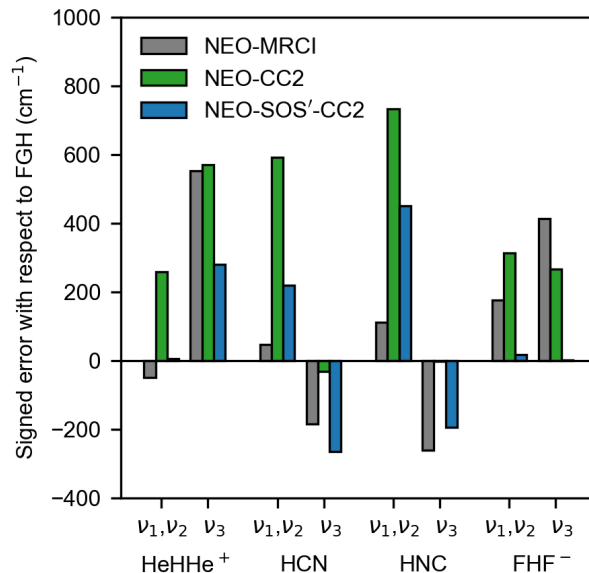

Figure S1: Signed error of the fundamental frequencies with respect to FGH values for four molecules. These frequencies correspond to the degenerate bending modes ( $\nu_1, \nu_2$ ) and the stretching mode ( $\nu_3$ ) in each molecule. The NEO-MRCI results obtained from Ref. 1 are shown in gray, the NEO-CC2 results are shown in green, and the NEO-SOS'-CC2 with  $c_{\text{ep}}^{\text{gs}} = 1.0$  and  $c_{\text{ep}}^{\text{ex}} = 8.0$  results are shown in blue, appearing in this order from left to right. Note that the error of NEO-CC2 for the stretching mode of HNC and the error of NEO-SOS'-CC2 for the stretching mode of FHF<sup>-</sup> are too small to be visible on this scale.

### S3 HCN with different conventional basis sets

In this section, we present the excitation energies of HCN using basis sets that allow direct comparison of the NEO-CC2 and NEO-SOS'-CC2 results to the NEO-EOM-CCSD results in Ref. 2. In these calculations, the cc-pVDZ electronic basis set is used for C and N, whereas the cc-pVDZ, cc-pVQZ, and cc-pV6Z electronic basis sets and the PB4-F2a' protonic basis set are used for the quantum hydrogen. Results are reported in Table S3.

Table S3: First four protonic excited states for HCN. The states are labeled according to quanta in the protonic vibrational modes  $(\nu_1, \nu_2, \nu_3)$ , where  $\nu_1$  and  $\nu_2$  are degenerate bending modes and  $\nu_3$  is the stretching mode. The NEO-SOS'-CC2 results are given with different scaling factors, reported as  $(c_{\text{ep}}^{\text{gs}}, c_{\text{ep}}^{\text{ex}})$ . All values are given in  $\text{cm}^{-1}$ .

| Basis | Method                     | (1,0,0)/(0,1,0) | (1,1,0) | (2,0,0)/(0,2,0) | (0,0,1) |
|-------|----------------------------|-----------------|---------|-----------------|---------|
| DZ    | FGH Reference <sup>a</sup> | 634             | 1261    | 1277            | 3173    |
| DZ/DZ | NEO-EOM-CCSD <sup>a</sup>  | 3024            | 5621    | 6041            | 4376    |
|       | NEO-TDHF <sup>a</sup>      | 3152            | 9553    | 9881            | 4570    |
|       | NEO-CC2                    | 3231            | 6196    | 6575            | 4546    |
|       | NEO-SOS'-CC2 (0.91,1.0)    | 2985            | 5910    | 6325            | 4283    |
|       | NEO-SOS'-CC2 (1.0,8.0)     | 3122            | 6123    | 6570            | 4386    |
| DZ/QZ | NEO-EOM-CCSD <sup>a</sup>  | 1749            | 3637    | NA <sup>b</sup> | 3768    |
|       | NEO-TDHF <sup>a</sup>      | 1942            | 9487    | 9923            | 3678    |
|       | NEO-CC2                    | 2187            | 4552    | 5090            | 3869    |
|       | NEO-SOS'-CC2 (0.91,1.0)    | 1724            | 3947    | 4609            | 3381    |
|       | NEO-SOS'-CC2 (1.0,8.0)     | 1690            | 3906    | 4864            | 3444    |
| DZ/6Z | NEO-TDHF <sup>a</sup>      | 876             | 9361    | 9781            | 3286    |
|       | NEO-CC2                    | 2076            | 4651    | 5134            | 3814    |
|       | NEO-SOS'-CC2 (0.91,1.0)    | 1541            | 3962    | 4579            | 3247    |
|       | NEO-SOS'-CC2 (1.0,8.0)     | 1364            | 3796    | 4802            | 3228    |

<sup>a</sup> FGH, NEO-EOM-CCSD and NEO-TDHF values obtained from Ref. 2.

<sup>b</sup> Mode was not detected with NEO-EOM-CCSD calculation due to having zero oscillator strength.

## References

- (1) Malbon, C. L.; Hammes-Schiffer, S. Nuclear-Electronic Orbital Multireference Configuration Interaction for Ground and Excited Vibronic States and Fundamental Insights into Multicomponent Basis Sets. *J. Chem. Theory Comput.* **2025**, *21*, 3968–3980.
- (2) Pavošević, F.; Tao, Z.; Culpitt, T.; Zhao, L.; Li, X.; Hammes-Schiffer, S. Frequency and Time Domain Nuclear-Electronic Orbital Equation-of-Motion Coupled Cluster Methods: Combination Bands and Electronic-Protonic Double Excitations. *J. Phys. Chem. Lett.* **2020**, *11*, 6435–6442.
